# Supplementary material for: Classifying soft self-assembled materials via unsupervised machine learning of defects
Source: arXiv:2112.08044 ancillary file (2021-12-15)
Supplement: Supplementary file 1 [file Supporting_Information.pdf]

# Supporting Information for: Classifying soft self-assembled materials via unsupervised machine learning of defects

Andrea Gardin[1], Claudio Perego[2], Giovanni Doni[2], and Giovanni M. Pavan[1,2]

[1]Department of Applied Science and Technology, Politecnico di Torino, Corso Duca degli Abruzzi 24, I-10129 Torino, Italy
[2]Department of Innovative Technologies, University of Applied Sciences and Arts of Southern Switzerland, Polo Universitario Lugano - Campus Est, Via la Santa 1, CH-6962 Lugano - Viganello, Switzerland

## S1 Additional figures

### S1.1 Schematic workflow

Comparison analyses presented in the main text follow a custom recipe that can be schematically summarized in Fig. S1. In Fig. S2A-C the treatment of the data and its transformations from the MD trajectory conformations to the clustering of molecular motifs is presented with more detail ; this scheme holds both when treating "global"-SOAP descriptors like the *frame*-average and the *simulation*-average (defined in the Methods section in the main text).

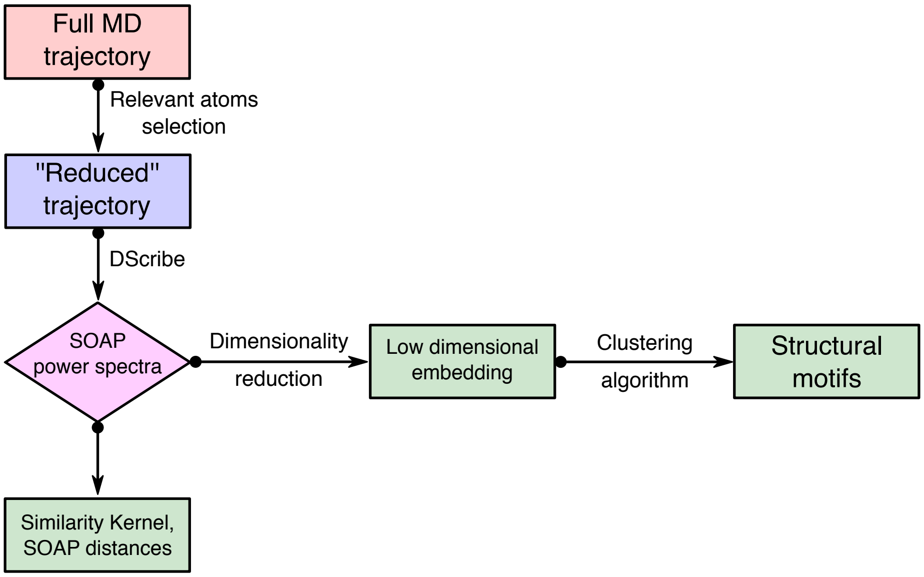


Figure S1: Step-by-step schematic workflow of the comparative analysis method.

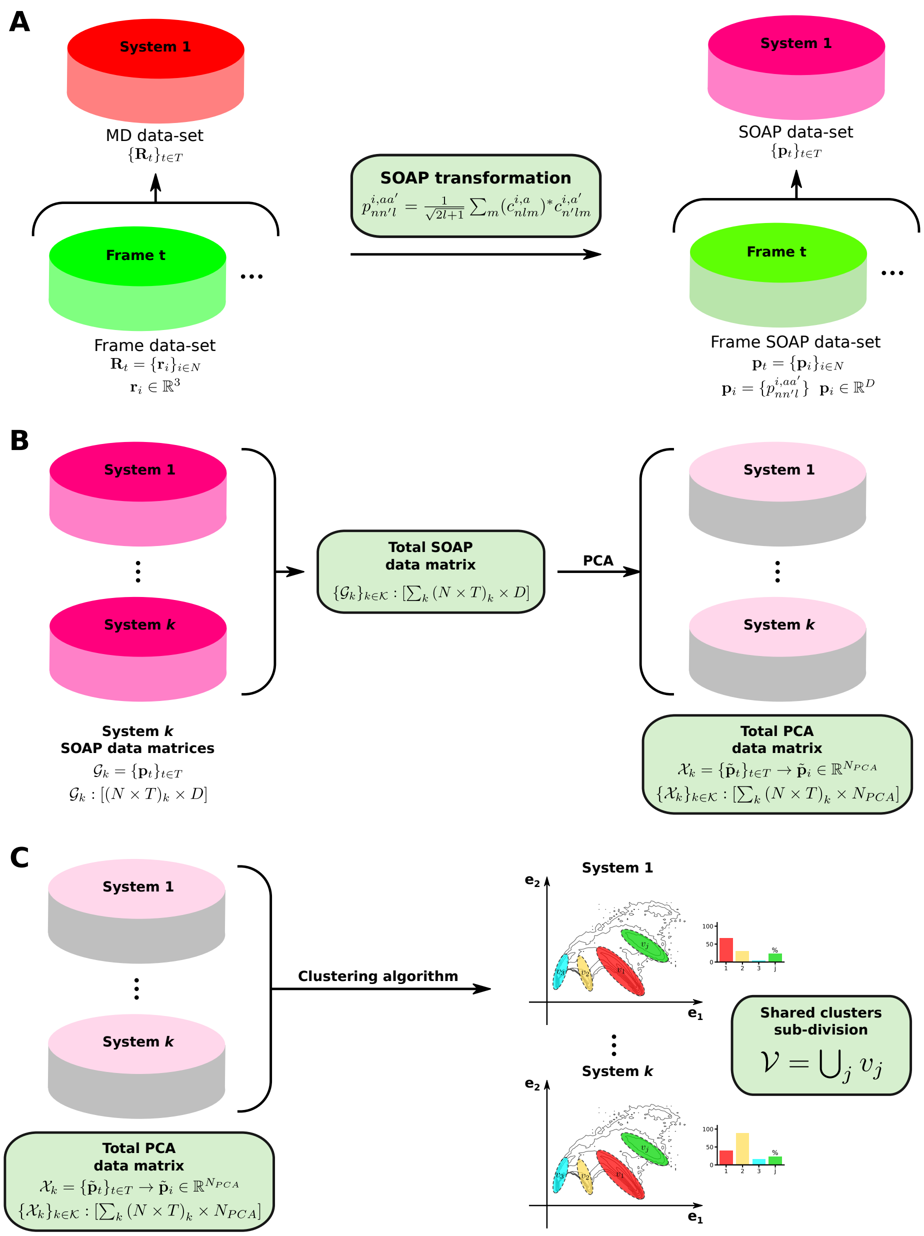


Figure S2: In-depth schematic workflow of the comparative analysis method: (A) MD trajectory data representations in terms of SOAP feature vectors for for each chosen "center" of a system and for each chosen frame of its MD trajectory. (B) Merging of SOAP datasets from multiple systems and computation of the PCA over the resulting merged data-set. (C) From the PCA data-set a clustering algorithm is applied to identify the molecular motifs and characterize the similarities among the systems.

## S1.2 PC analysis variance.

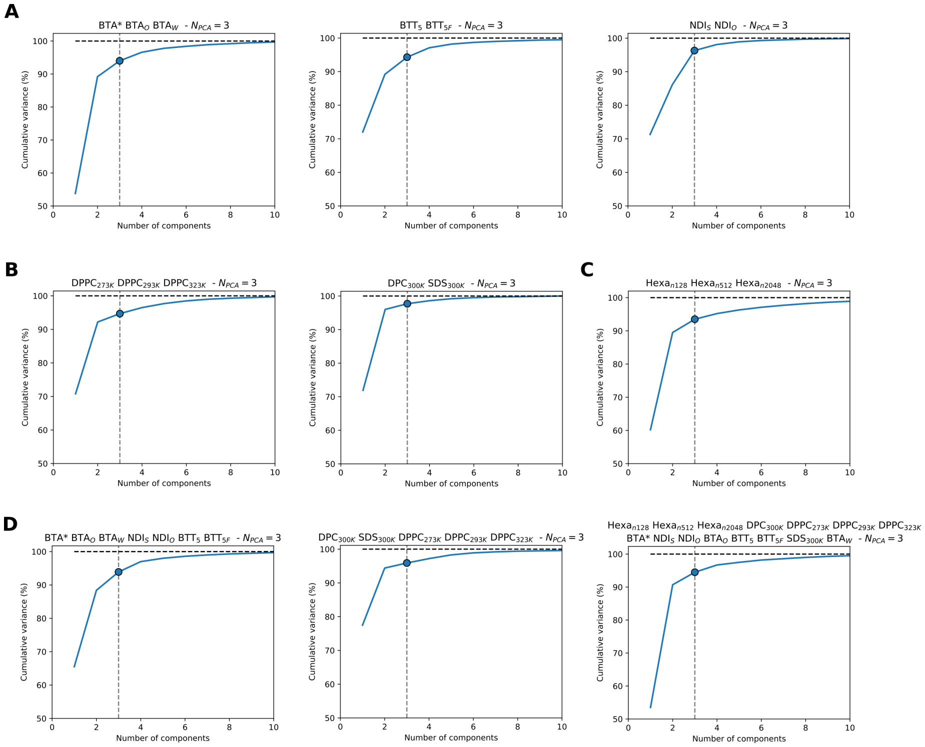


Figure S3: PCA variance for all the systems studied in the main text, as a function of the number $N_{PCA}$ of principal components retained in the dimensionality reduction. The variance corresponding to $N_{PCA} = 3$ is highlighted. (A) Supramolecular polymers, (B) micelles and lipid membranes, (C) nanoparticles, (D) joint dataset of respectively (from left to right) all the supramolecular polymers, all the micelles and lipid membranes, and all the systems combined. The systems included in the analysed dataset are listed at the top of each plot.

## S1.3 Radial distribution function

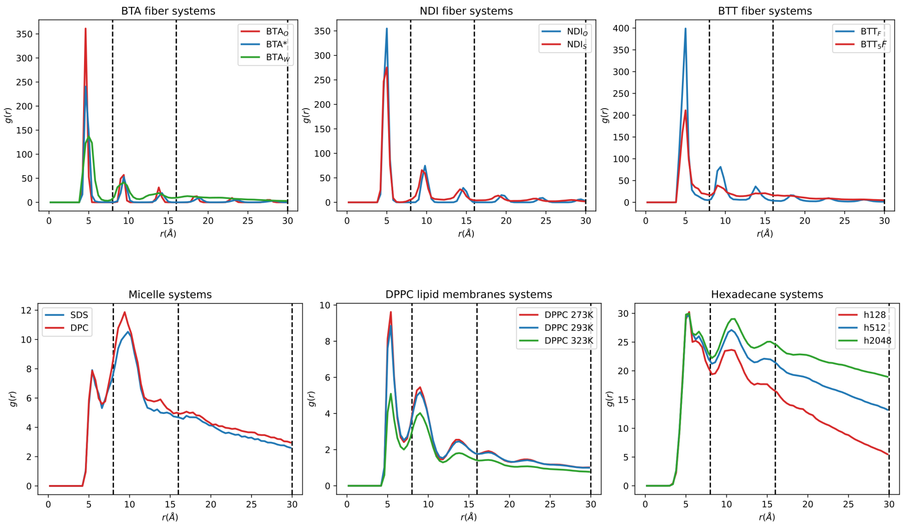


Figure S4: Radial distribution functions for each system studied in this work (solid lines). The dashed vertical lines indicate the three different `rcut` values employed in our analyses, namely 8, 16, 30 Å.

## S1.4 Systems comparison at rcut $= 1.6, 3.0$ nm

Following the definition of the SOAP[1] descriptor, changing the cutoff `rcut` directly changes the fingerprint of the atomic environment surrounding each center in the system. This change affects more significantly the high-dimensional aggregates, where the coordination of centers scales increasing with the cutoff radius, as compared to one-dimensional supramolecular polymers (see also Fig.S4 for reference). The overall fingerprints obtained via SOAP descriptors appear to be more rich in information, since every small difference in the coordination shells leads to a different SOAP feature vector. In this sense at higher cutoff radius we obtain a larger data variance, after dimensional reduction, corresponding to the inclusion of higher coordination shells in the descriptor definition. In Fig.S5 the areas corresponding to the green and red clusters reflect respectively the surface of the membranes/micelles and the core of the nanoparticles; In Fig.S6 the areas corresponding to the blue and red clusters reflect respectively the core of the nanoparticles.

Given that the "local"-SOAP feature vectors account for all these little differences as they should, the "global"-SOAP descriptor still carries an averaged fingerprint of the whole structural aggregates, moreover, translating it to mutual distances (using the definition of SOAP metrics) we observe that the trend is more or less conserved along the cutoff values (Fig. 6 of main text).

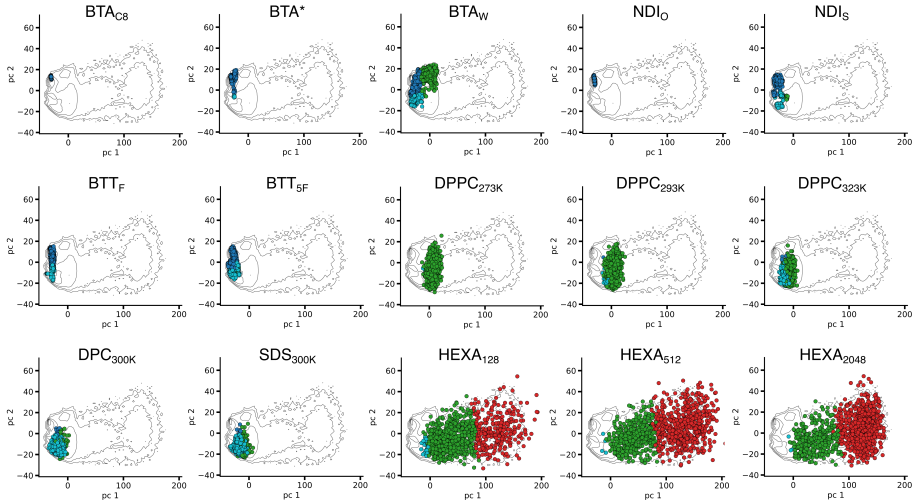


Figure S5: Comparison at `rcut` = 1.6 nm. Each panel reports the PC scatter plot of SOAP feature vectors relative to a single system (in colour) superimposed over the SOAP feature vectors of the global dataset (black contour plot). The colours indicate the molecular motifs detected by the PAMM clustering algorithm.

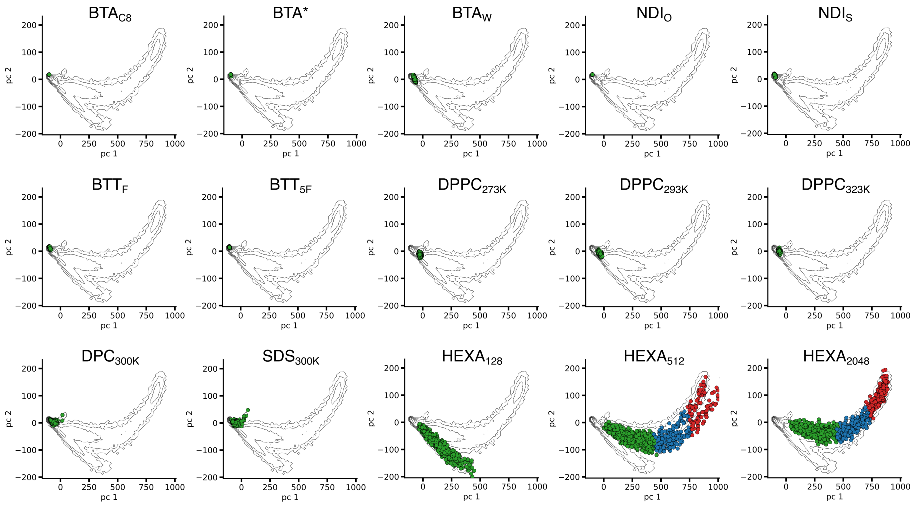


Figure S6: Comparison at `rcut` = 3.0 nm. Each panel reports the PC scatter plot of SOAP feature vectors relative to a single system (in colour) superimposed over the SOAP feature vectors of the global dataset (black contour plot). The colours indicate the molecular motifs detected by the PAMM clustering algorithm.

## S1.5 SDS+DPC micelles analysis

In Fig. S7 we report the SOAP+PAMM analysis applied to the dataset composed by the two different micellar systems (SDS and DPC). The PCA projection along the first two components does not show a particularly interesting "fingerprint", as confirmed by the clustering algorithm. Looking at the molecular microstates detected by the PAMM algorithm (see Ref.[2] for the details of the method) minor differences in the SOAP environments are identified, due mostly to variations in the mutual organization of monomers (Fig. S7A). This distinction is hardly to be attributed to a different phase behavior. This is confirmed by the statistical analysis of the dynamic between these micro-states, which exhibits fast reshuffling between these molecular motifs, so that they can be identified into a single macro-state (Fig. S7B).

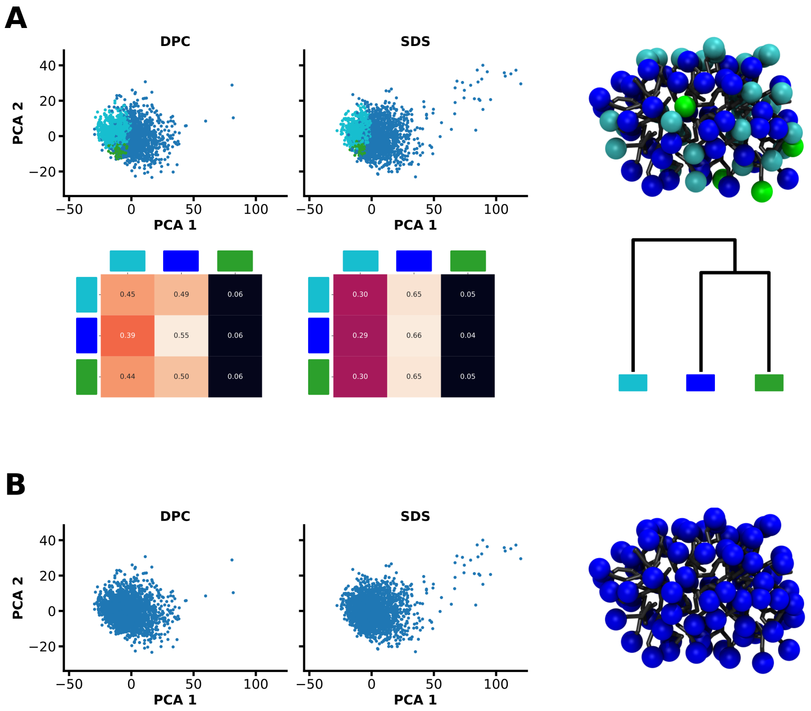


Figure S7: SOAP+PAMM analysis results for the DPC and SDS micelles.

## S1.6 DPPC lipid membranes analysis

Fig. S8 reports results for the SOAP+PAMM analysis of the DPPC lipid membranes data, showing how the `rcut` in the SOAP descriptor calculation affects the separation of the two environments belonging to the liquid and gel phases. A large cutoff radius is needed in order to catch enough detail to better differentiate the local environments.

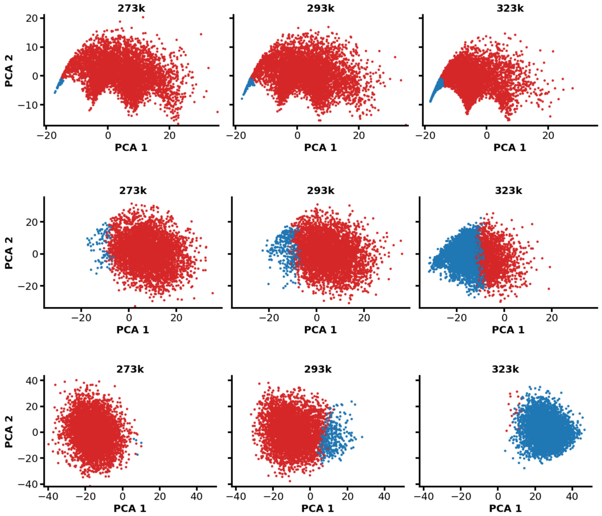


| ($r_{cut} = 8\AA$) | DPPC$_{273K}$ | DPPC$_{293K}$ | DPPC$_{323K}$ |
|---|---|---|---|
| Red | 0.993 | 0.983 | 0.831 |
| Blue | 0.007 | 0.016 | 0.169 |

| ($r_{cut} = 16\AA$) | DPPC$_{273K}$ | DPPC$_{293K}$ | DPPC$_{323K}$ |
|---|---|---|---|
| Red | 0.985 | 0.943 | 0.665 |
| Blue | 0.015 | 0.056 | 0.335 |

| ($r_{cut} = 30\AA$) | DPPC$_{273K}$ | DPPC$_{293K}$ | DPPC$_{323K}$ |
|---|---|---|---|
| Red | $< 0.999$ | 0.946 | 0.004 |
| Blue | $> 0.001$ | 0.054 | 0.996 |

Figure S8: SOAP+PAMM analysis results for the DPPC lipid membranes systems using different `rcut` values of 8, 16, 30Å.

## S1.7 DPPC+SDS+DPC comparison

Fig. S9 reports the results for the combined analysis of the DPPC, DPC, and SDS systems. In the PCA scatterplots the micelles systems position themselves closer to the liquid DPPC membrane (at temperature of 323 K), indicating higher similarity of the local environments populated by these systems, although a quantitative difference is signaled by the comparison of averaged SOAP data and by the calculation of the relative SOAP distances.

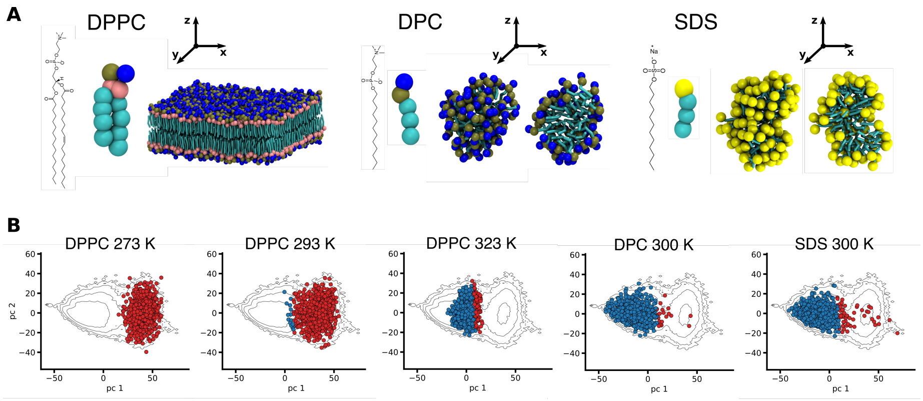


Figure S9: SOAP+PAMM analysis for the 2D supramolecular aggregates (DPPC, DPC and SDS).

## S1.8 Choice of the SOAP centers

Fig. S10 reports the SOAP centers defined for each of the monomer models studied in the present work.

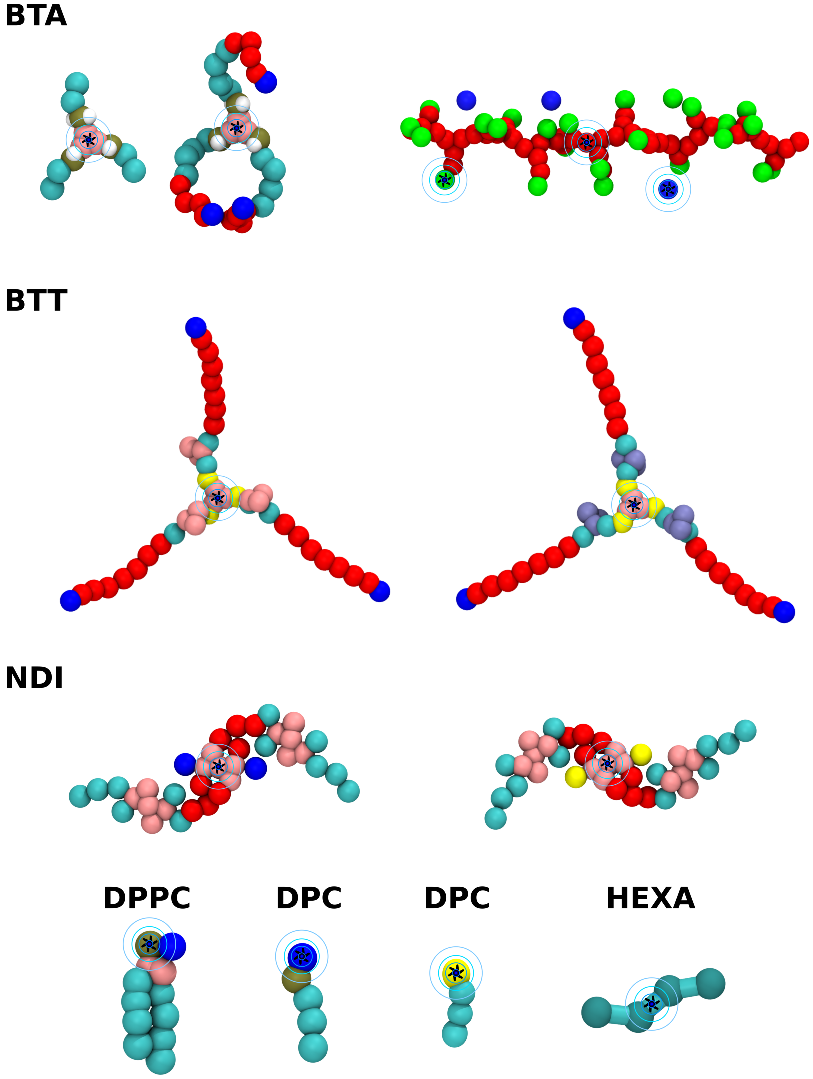


Figure S10: SOAP center defined in the analysis, indicated as a black star for each of the studied monomer models. The light blue circles indicate the different choices of `rcut` used in this work, namely 0.8, 1.6, 3.0 nm.

# References


[1] Bartók, A. P.; Kondor, R.; Csányi, G. *Phys. Rev. B* **2013**, *87*, 184115.

[2] Gasparotto, P.; Meißner, R. H.; Ceriotti, M. *J. Chem. Theory Comput.* **2018**, *14*, 486–498, PMID: 29298385.
